# Supplementary material for: Evidence for the decay $B^0\to J/\psi \omega$ and measurement of the relative branching fractions of $B^0_s$ meson decays to $J/\psi\eta$ and $J/\psi\eta^{'}$
Source: arXiv:1210.2631 source file (2012-10-09)
Supplement: Supplementary file 3 [file supplementary-app.tex]

\clearpage

\section{Supplementary Material}
\label{sec:Supplementary-App}

{\bf This appendix includes supplementary material that will be made
  available on CDS during the review phase but will not appear in the
  final version of the paper.}

\begin{figure}[!htb]
  \begin{center}
    \includegraphics[scale=0.65,bb=50 300 580 700,clip=true]{Roger-plot}
    \vspace*{-1.0cm}
  \end{center}
  \caption{
    \small %captions should be a little bit smaller than main text
    This plot compares our result to those from other experiments.}
  \label{fig:roger}
\end{figure}

\clearpage
